# Supplementary material for: Corners for Layout: End-to-End Layout Recovery from 360 Images
Source: arXiv:1903.08094 source file (2019-03-25)
Supplement: Supplementary file 1 [file supplementarymaterial.tex]

\appendix

\subsection{Atrous}

\subsection{Special cases}
\subsubsection{Ground truth analysis}

\subsubsection{Non-Manhattan}

\subsection{Qualitative Results}
\subsubsection{SUN360 dataset}

\subsubsection{Stanford 2D-3D dataset}
